# Supplementary material for: High harmonics from backscattering of delocalized electrons
Source: arXiv:2102.11208 ancillary file (2022-03-11)
Supplement: Supplementary file 1 [file chain-suppl.pdf]

# Supplement "High harmonics from backscattering of delocalized electrons"

Chuan Yu, Ulf Saalmann and Jan M Rost

The laser-driven quiver motion in a periodic potential is discussed by means of a Kane model for the band structure.

In the Kane model [1] the band structure is approximated up to a constant by

$$E(k) = E_{\mathrm{b}}\sqrt{1+k^2/(m_*E_{\mathrm{b}})}, \tag{S1}$$

with $E_{\mathrm{b}}$ a characteristic band energy and $m_*$ the effective mass. This model represents the real band structure extremely well, as can be seen in Fig. S1. The group velocity in this band reads

$$\frac{\mathrm{d}}{\mathrm{d}k}E(k) = \frac{k/m_*}{\sqrt{1+k^2/k_*^2}} \qquad \text{with} \quad k_* \equiv \sqrt{m_*E_{\mathrm{b}}}, \tag{S2}$$

which shows that, particularly if $k$ is larger than the characteristic band momentum $k_*$, the free-particle velocity $k/m_*$, given by the numerator, is modified such that it saturates at a maximal value of $k_*/m_*$. Note that $k_*$ characterizes the point where the band dispersion changes from parabolic to quasi-linear behavior.

Assuming that $k$ follows the oscillating vector potential $A(t)=A_0\sin(\omega t)$, one can calculate the quiver position of a particle starting at $x(t_0)=0$ by

$$x(t) = \frac{A_0/\omega}{m_*}\int_{\varphi_0}^{\varphi}\mathrm{d}\varphi' \frac{\sin\varphi' - \sin\varphi_0}{\sqrt{1+a^2[\sin\varphi' - \sin\varphi_0]^2}} \qquad \text{with} \quad a \equiv \frac{A_0}{k_*}. \tag{S3}$$

The dimension-less $a$ is the "normalized" vector potential. The integration limits are $\varphi_0=\omega t_0$ and $\varphi=\omega t$, respectively. Apparently the conventional (free-space) quiver motion and thus its amplitude are modified. The modification of the amplitude $A_0/\omega$ are caused by both the effective mass $m_*$ and the integral over $\varphi'$.

There is no simple analytical expression for the integral in Eq. (S3). Therefore, we show the result of the integral for selected values of $t_0$ in Fig. S2. A small value of $a=1/3$, left column of Fig. S2, implies motion in the harmonic region of the band. The dynamics is similar to the free motion in the case of gas-phase atoms. A large value of $a=3$, however, as used in right column of Fig. S2, probes the linear part of the band structure. In this case the motion is notably different with respect to the atomic case. It is partly linear, which is a consequence of the upper limit for the velocity discussed for Eq. (S2), and the quiver amplitude is considerably smaller than $A_0/m_*\omega$. In all cases the quiver motion and also its amplitude depend on the initial phase $\varphi_0$, something that is not seen in the atomic case.

For the special case of $t_0=0$ the quiver amplitude is maximal, as can be seen in the lower row of Fig. S2, and the integral in (S3) is a simple analytical expression, namely $x_{\mathrm{q}}=\xi_a A_0/m_*\omega$ with

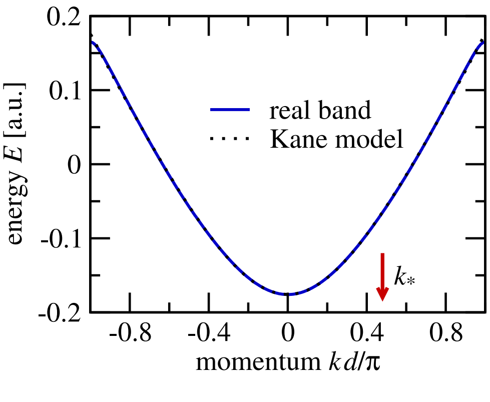


Figure S1: Kane model (S1) in comparison to the real structure of the 1st conduction band. The model (black dotted line) perfectly matches the band (blue solid line) except from tiny deviations at the Brillouin-zone boundaries. The characteristic band momentum $k_*$ is shown by the red arrow.

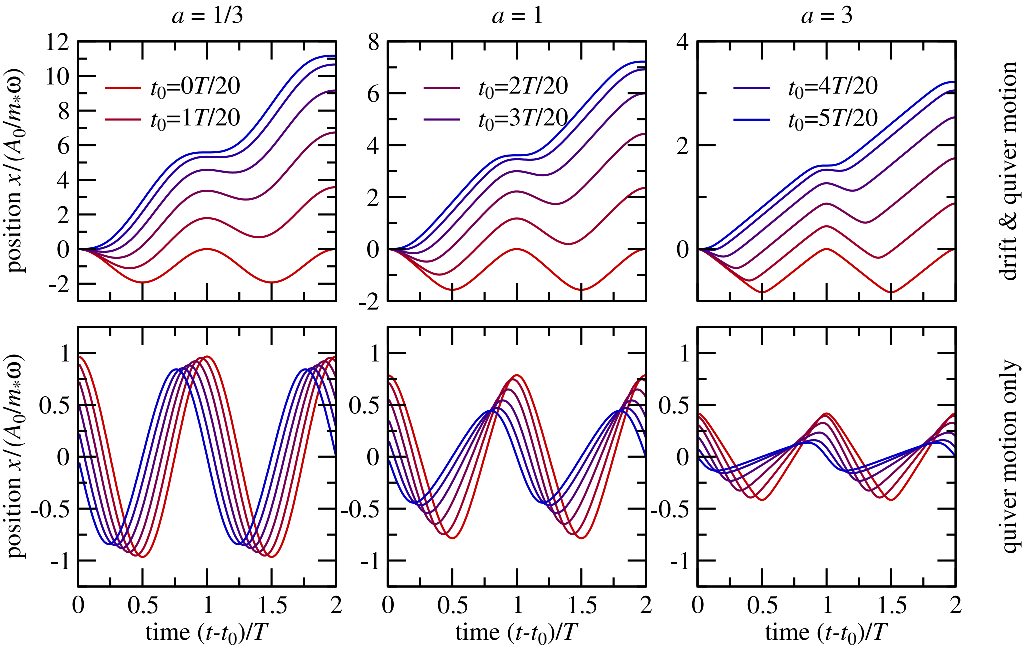


Figure S2: Motion according to the integral (S3) for three values of $a$ and six initial times $t_0$ (upper row), and quiver motion only, i. e. the drift motion substracted (lower row), for two laser cycles each. Note the different vertical scales in the upper row.

$\xi_a \equiv \arctan(a)/a$. The prefactor $\xi_a$ reduces the quiver amplitude and takes the values $\xi_0 = 1$, $\xi_1 = \pi/4$ and $\xi_{a\to\infty} = \pi/2a$, respectively. For the chains considered in the main text it is $E_\mathrm{b} = 0.239$ and $m_* = 0.167$, which results for $A_0 = 0.21$ in $a = 1.05$. Due to the small effective mass $m_*$, the quiver amplitude of the conduction-band electron is much larger than the free-electron quiver radius $A_0/\omega$ in the atomic case. This is only weakly compensated by the factor $\xi_{1.05} = 0.77$ in our considered scenario.

[1] E. O. Kane, *Band structure of indium antimonide*. J. Phys. Chem. Solids **1**, 249 (1957).
